# Supplementary material for: S=1/2 quantum critical spin ladders produced by orbital ordering in Ba2CuTeO6
Source: arXiv:1511.01477 ancillary file (2015-11-04)
Supplement: Supplementary file 1 [file SupplementalMaterial_Ba2CuTeO6_Gibbs_etal.pdf]

# Supplemental Material

# for

# *S=1/2 quantum critical spin ladders produced by orbital ordering in $Ba_2CuTeO_6$*

A. S. Gibbs, A. Yamamoto, A. N. Yaresko, K. S. Knight, H. Yasuoka, M. Majumder, M. Baenitz, P. J. Saines, J. R. Hester, D. Hashizume, A. Kondo, K. Kindo, and H. Takagi

## Structure determination

X-ray single crystal structure solution was performed on data acquired using a Rigaku AFC-8 diffractometer with molybdenum $K_\alpha$ radiation at $T$ = 296 K (Table S1).

**Table S1:** X-ray single crystal diffraction structure solution results for $T$=296 K.

| Space Group: *C2/m*, No. 12<br>$R_1$=0.0435, $wR_2$=0.1271, $\chi^2$=1.193, 58 var.<br>$a$ = 10.2444(3) Å, $b$ = 5.7315(2) Å, $c$ = 10.1055(5) Å, β = 108.019(3)° | | | | | |
|---|---|---|---|---|---|
| Site | Wyckoff Position | x | y | z | $U_{iso}$ (Å$^2$) |
| Ba1 | 4i | 0.12919(3) | 0 | 0.37910(3) | 0.01776(11) |
| Ba2 | 4i | 0.28313(3) | 0 | 0.84996(4) | 0.01879(11) |
| Te1 | 2a | 0 | 0 | 0 | 0.01419(11) |
| Te2 | 2d | 0 | 0.5 | 0.5 | 0.01478(12) |
| Cu1 | 4i | -0.09331(7) | 0.5 | 0.21497(7) | 0.01659(13) |
| O1 | 4i | 0.1328(4) | 0.5 | 0.3998(5) | 0.0202(6) |
| O2 | 8j | -0.1046(3) | 0.7283(5) | 0.3687(3) | 0.0198(4) |
| O3 | 4i | 0.3177(5) | 0.5 | 0.8754(5) | 0.0243(7) |
| O4 | 8j | 0.0508(3) | 0.7603(5) | 0.8905(4) | 0.0267(6) |

High-resolution neutron diffraction data from HRPD at ISIS (UK) was consistent with this assignment and revealed the presence of a high-temperature Jahn-Teller transition at $T$ = 847 K and a second order transition to $P\bar{1}$ at $T$ = 287 K.

The polycrystalline samples used in this work were phase pure as determined by x-ray and neutron diffraction. Powder x-ray diffraction of crushed single crystals confirmed the absence of impurity phases.

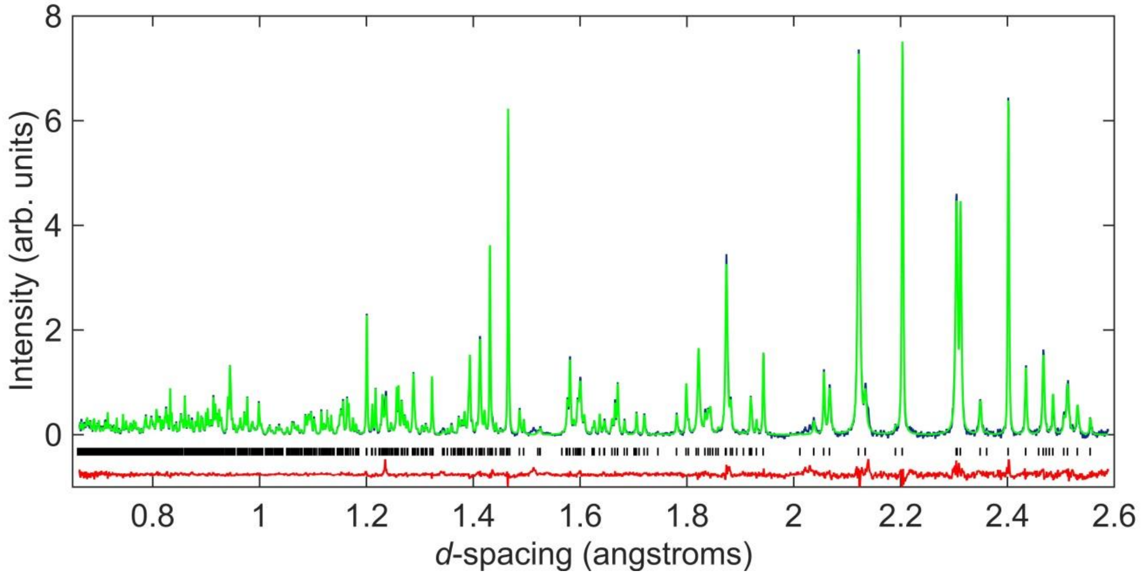


**Figure S1** Rietveld refinement results of 300 K HRPD (bank 1) neutron diffraction data for $Ba_2CuTeO_6$ using GSAS profile function 4. The blue line indicates the raw data, the green line the Rietveld refinement fit and the red line the difference profile. Black tick marks indicate peak positions for the *C*2/*m* phase. $R_{wp}$=0.0239, $\chi^2$=2.199 for 74 variables.

## Electronic Structure Calculations:

The band structure calculations were done for the high temperature *C*2/*m* structure of $Ba_2CuTeO_6$ using the LSDA+U method with a range of *U*=4-8 eV and *J*=1 eV which is close to the value estimated from LSDA. The total energy $E(\mathbf{q}, \varphi)$ was calculated as a function of a wave vector $\boldsymbol{q}$ and of an angle φ between spins of two $Cu^{2+}$ ions in the *C*2/*m* unit cell for a number of spin-spiral structures. Then, effective exchange coupling constants $j_i$ were evaluated by fitting $E(\boldsymbol{q}, \varphi)$ to a classical Heisenberg model [1,2]. For simplicity, only spirals with $\boldsymbol{q} = (0, q_y, 0)$ were considered.

**Table S2:** Exchange parameters $j_i$ (meV) obtained from the fits assuming Cu spin of *S*=1/2

| | ***J*** | ***J'*** | ***j*₁** | ***j*₂** | ***j*₃** |
|---|---|---|---|---|---|
| ***J*, *J'*, $j_1$** | 32.0 | 31.2 | -0.06 | | |
| ***J*, *J'*, $j_1$-$j_3$** | 33.8 | 33.0 | 1.7 | -1.9 | -1.6 |

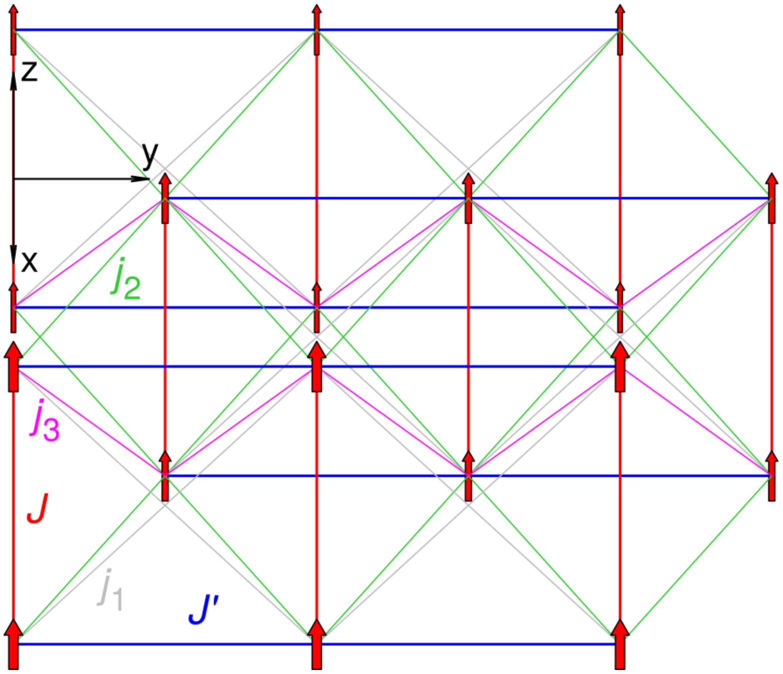


**Figure S2** Intra-ladder *J,J',j₁* and inter-ladder $j_2$, $j_3$ exchange coupling constants used to fit the calculated ***q***-dependence of the total energy. The distances between Cu spins coupled by $j_i$ are $d_J$=5.23 Å, $d_{J'}$=5.72 Å, $d_1$=7.75 Å, $d_2$=5.86 Å, $d_3$=5.35 Å

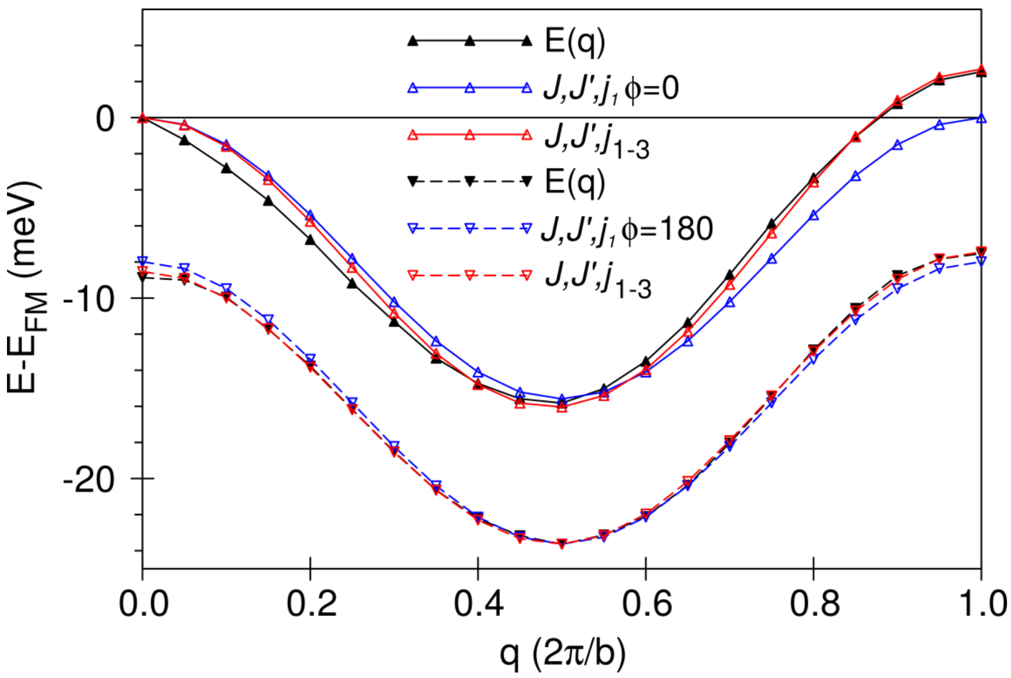


**Figure S3** Calculated E(**q**, 0) (solid black line) and E(**q**, π) (dashed black line) plotted together with the magnetic energies Eq. (1) with $j_i$ obtained from least-square fits to the $J,J',j_1$ (blue lines) and $J,J',j_{1-3}$ (red lines) Heisenberg models.

## Magnetic Susceptibility:

The chain model fits were performed for two parameters, $g$ and $J/k_B$, using Matlab for the $M/H$ data in the range 35 K < $T$ < 300 K using the Bonner-Fisher expression [3,4]:

$$\chi = \frac{N\mu_B^2 g^2}{k_B T}\frac{0.25+0.14995^{J}/_{k_B T}+0.30094(^{J}/_{k_B T})^2}{1+1.9862\left(^{J}/_{k_B T}\right)+0.68854(^{J}/_{k_B T})^2+6.0626(^{J}/_{k_B T})^3}.$$

Results are given in Table S3.

**Table S3:** The results of the Bonner-Fisher (chain) model fits.

| Bonner Fisher model | $g$ | $J/k_B$ (K) | Goodness of fit |
|---|---|---|---|
| *H //ab* | 2.061±0.007 | 57.64±0.53 | 0.9950 |
| $H\perp ab$ | 2.274±0.009 | 62.69±0.63 | 0.9923 |

The ladder model fits were performed for the $M/H$ data in the range 35 K < $T$ < 300 K with the Quantum Monte Carlo derived expressions for isolated ladders given in reference [5]. The fitted parameters were $g$, $J_1$, and the ratio $J'/J$. In the case of *H //ab* where $J/J'$ was not a robust fitting parameter it was fixed to the value obtained from the fit to the $H\perp ab$ data. The gap estimate was obtained but using expression (7) of the same paper. It should be noted that errors exist in some tables of coefficients in this preprint. The correctness of the coefficients used for our fits was confirmed by successful reproduction of the plots in the paper. The results from the fits are given in Table S4.

**Table S4:** The results of the isolated ladder model fits.

| Ladder model | $g$ | $J/k_B$ (K) | $J'/J$ | Goodness of fit |
|---|---|---|---|---|
| *H //ab* | 2.080 ±0.00 | 85.55 ± 1.04 | 0.981 ±0.019 | 0.9997 |
| $H\perp ab$ | 2.289 ±0.006 | 89.11± 0.58 | 0.98 | 0.9946 |

A fit of the isolated ladder model to data from a polycrystalline sample gives the results $J/k_B$ = 92.8±0.4 K, $g$=2.199±0.001 $J'/J$ = 0.886±0.011, the fit is shown in figure S4.

Our estimate for the upper limit of magnetic impurities was reached by postulating that the low temperature upturn for $T \leq 3$ K in $\chi(T)$ for $H\perp ab$ (seen in Fig. 2 of the main manuscript) could be due to Curie-like impurities. A best estimate was then made of the magnetic impurity content required to produce this upturn. This resulted in an estimated maximum impurity concentration of 0.07% $S$=1/2 impurities.

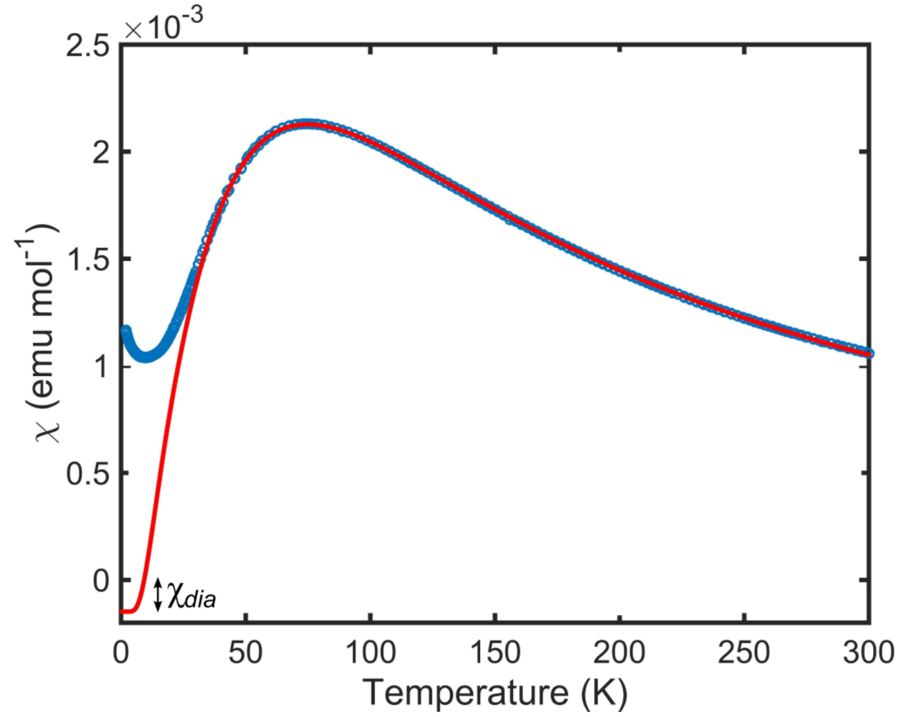


**Figure S4** The susceptibility of polycrystalline $Ba_2CuTeO_6$ measured in an applied magnetic field of 1 T. The red line shows the isolated ladder model fit.

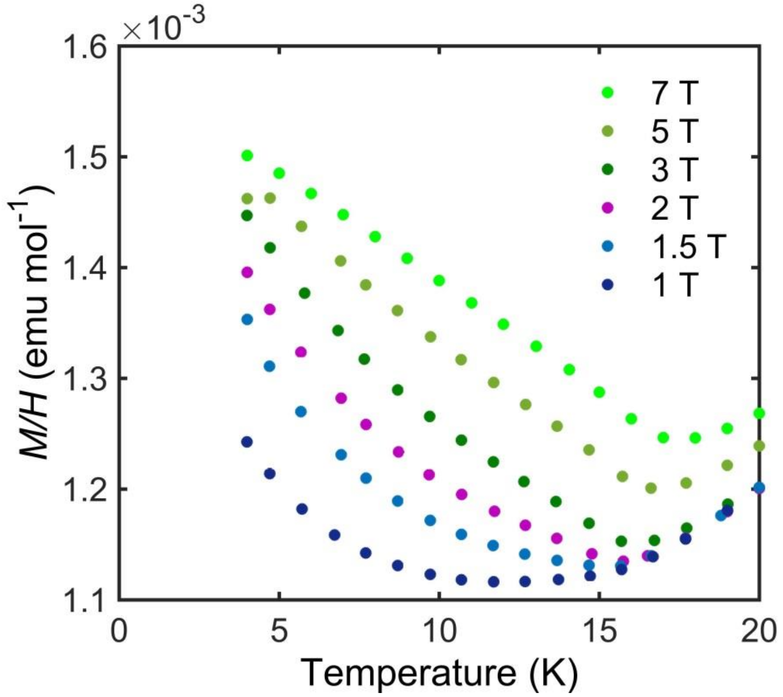


**Figure S5** The field dependence of *M/H* for a polycrystalline sample of $Ba_2CuTeO_6$.

## NMR:

The present $^{125}$Te powder NMR field sweep spectra were recorded using a conventional pulsed NMR spectrometer (Tecmag) at 55.44 MHz and at temperatures from 2 K to 300 K. The spectra were obtained by integrating the standard Hahn spin-echo transients from the $^{125}$Te nuclear spins ($I$=1/2, $\gamma_n$=13.45 MHz/T), recorded at constant field intervals. The spin lattice relaxation rate was obtained using the inversion recovery method in aligned arrays of single crystals in both $H\perp ab$ and $H||ab$ at the peak field of spectra. The observed recovery of the nuclear magnetization after an inversion pulse for $m$=+1/2↔$m$=-1/2 nuclear transition follows a single exponential function for all temperatures measured. Figure S6 (a) shows the temperature evolution of $^{125}$Te NMR spectra which could be consistently deconvoluted into two spectra associated with expected two Te sites with anisotropic (non-axial) transferred hyperfine interaction reflecting the triclinic crystal structure. The typical example is shown in Figure S6 (b) where the deconvoluted area of two spectra found to be consistent with the equal occupancy of two Te sites in the formula unit. The temperature dependence of isotropic part of the Knight Shift ($K_{iso}$) extracted from the singular positions ($K_a$, $K_b$ and $K_c$) for both of the sites are almost the same within experimental error which is depicted in Figure S6(c). Figure S7 shows the recovery curves for spin ½ nuclei, $M(t) = M(0)[1 - 2\exp\left(-\frac{t}{T1}\right)]$, at 14 and 26 K, where $M(t)$ and $M(0)$ is the nuclear magnetization at $t$=0 and $t$=∞ (the thermal equilibrium value), respectively.

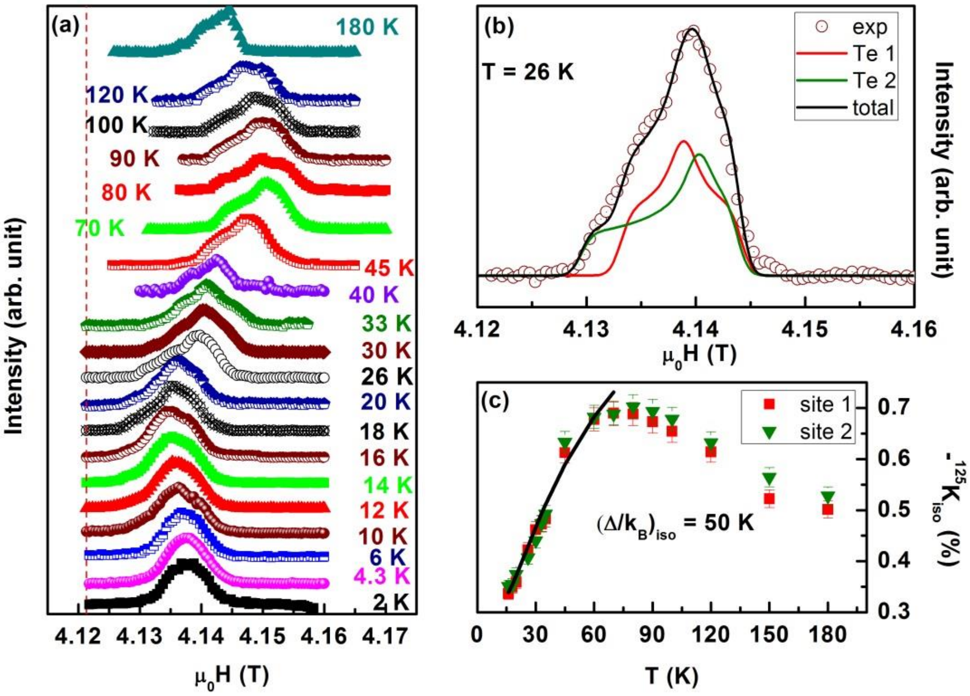


**Figure S6:** (a) Temperature dependence of $^{125}$Te NMR spectra. (b): Fitting of experimental spectra by simulation of two Te sites at 26 K, (c): temperature dependence of $K_{iso}$ (%) for both Te sites. The solid line corresponds to $K_{iso} = B\cdot\exp(-E_a/k_BT)$ fit.

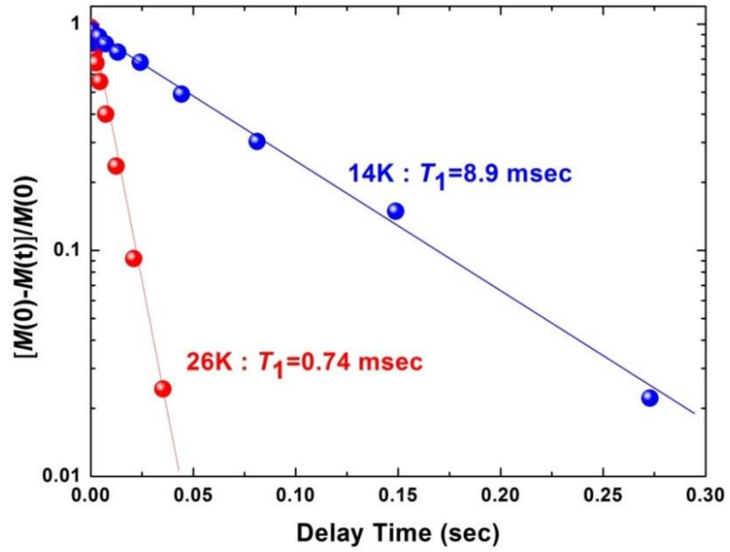


**Figure S7:** A typical example for the decay of the nuclear magnetization to the thermal equilibrium value at 14 K and 26 K. Solid lines are the best fit of the data to a single exponential relaxation process.

## Neutron Diffraction

Figures S8 and S9 show the powder neutron diffraction data from Echidna at the OPAL reactor (λ= 2.439 Å).

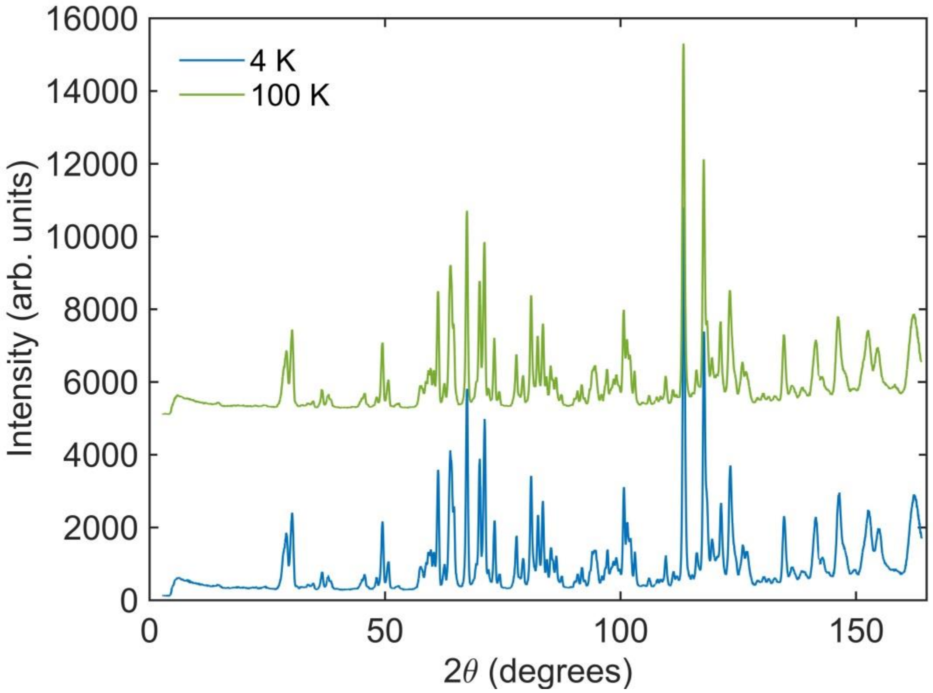


**Figure S8** The Echidna neutron diffraction data taken at $T$=4 K (blue) and $T$=100 K (green). The $T$=100 K data is offset by 5000 units. No magnetic Bragg peaks could be identified.

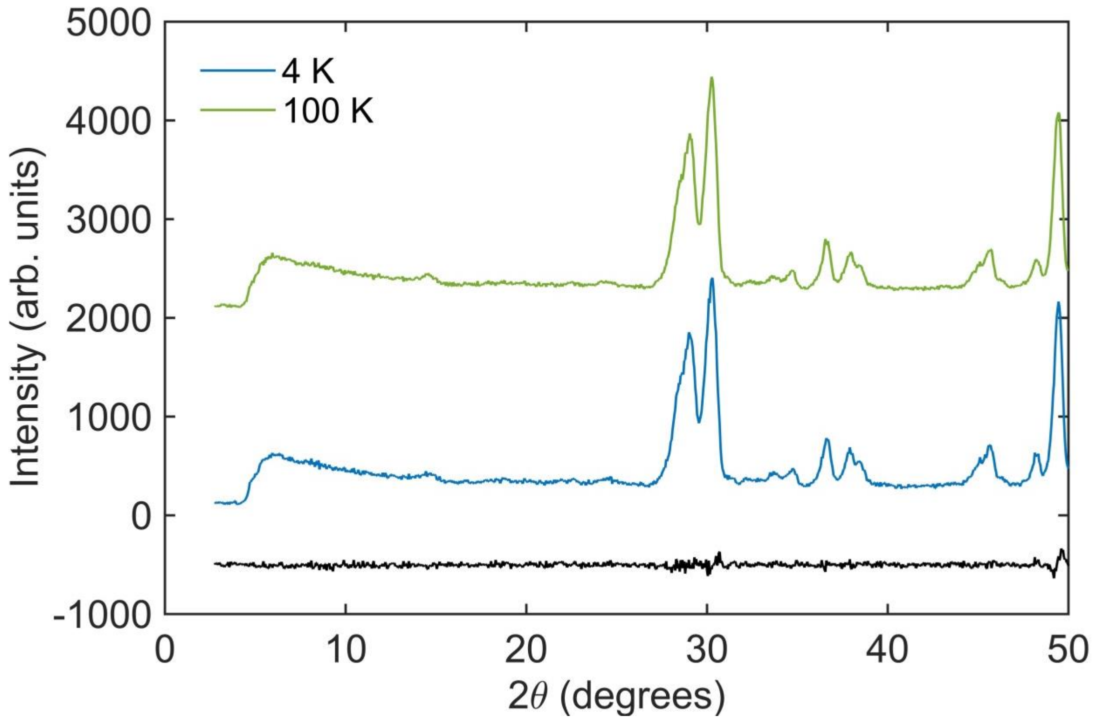


**Figure S9** The Echidna neutron diffraction data taken at $T$=4 K (blue) and $T$=100 K (green) with a difference curve shown in black. The $T$=100 K data is offset by 2000 units and the difference curve by -500 units.

## High Field Magnetization

High field magnetization data were taken at ISSP at $T$=4.2 K and under pulsed fields of up to 55 T using a static pickup coil (Figures S10, S11 and S12).

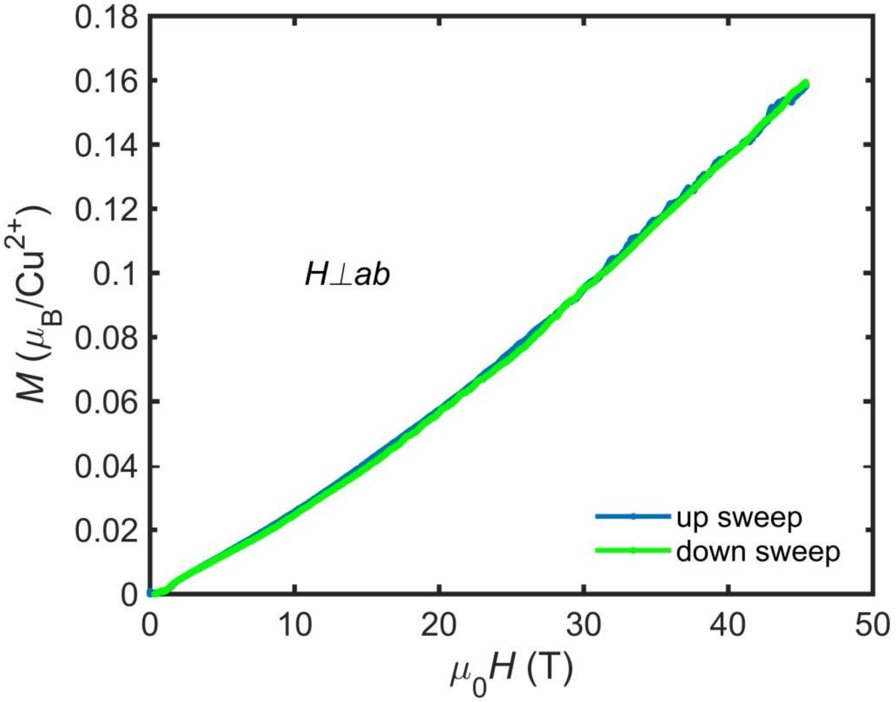


**Figure S10** High field magnetization data for $Ba_2CuTeO_6$ for $H \perp ab$.

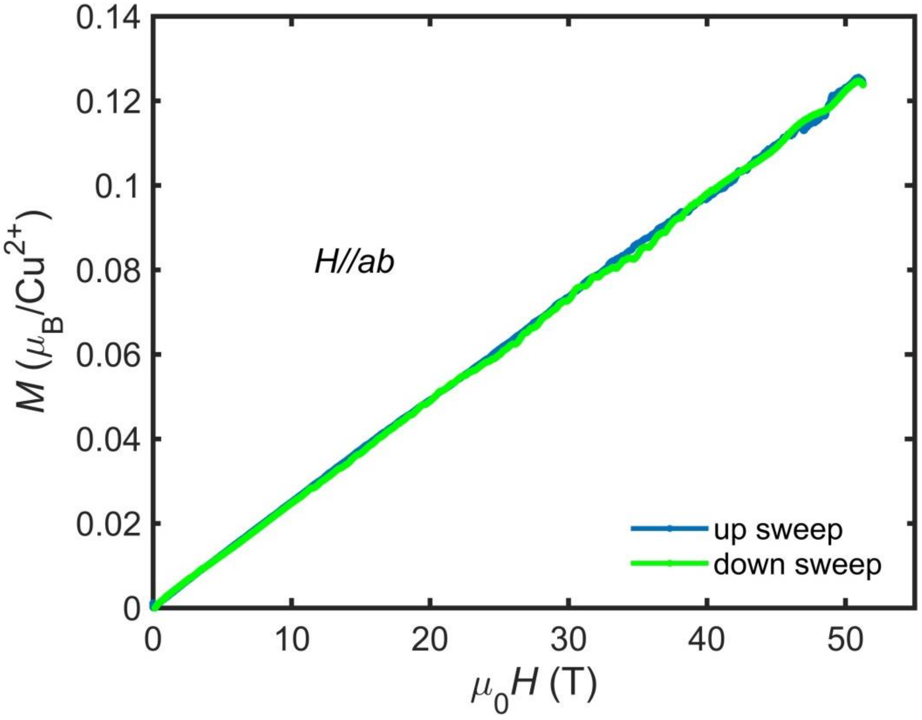


**Figure S11** High field magnetization data for $Ba_2CuTeO_6$ for *H // ab.*

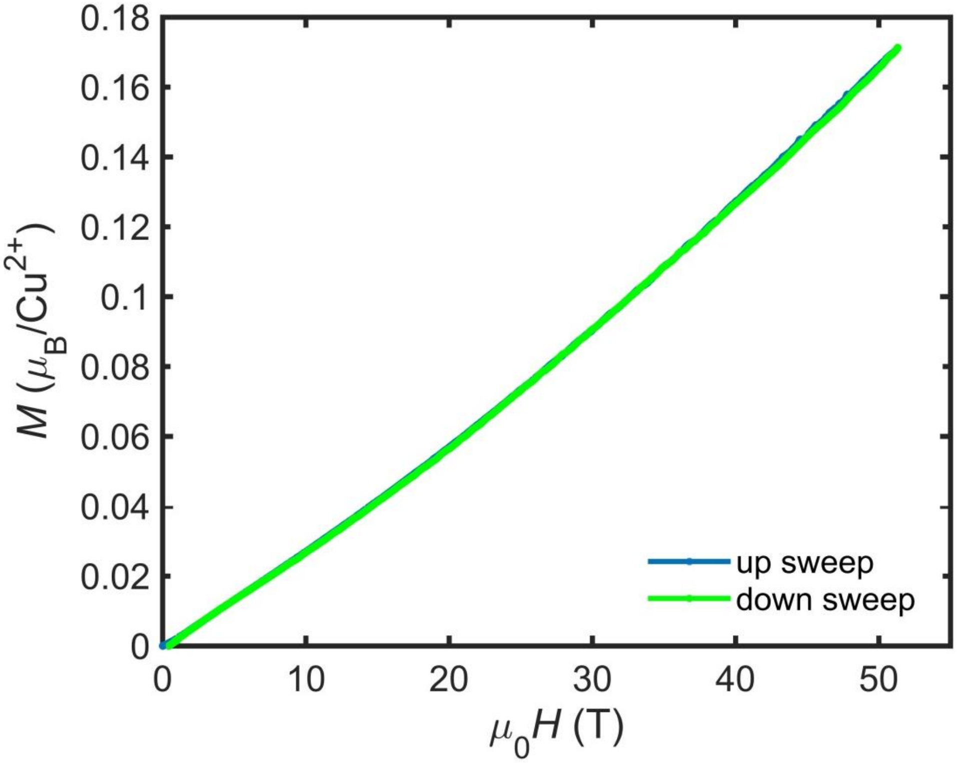


**Figure S12** High field magnetization data for polycrystalline $Ba_2CuTeO_6$.

**Specific Heat:**

Specific heat was measured using a 14 T Quantum Design PPMS with a $^3$He option (Figures S13 and S14).

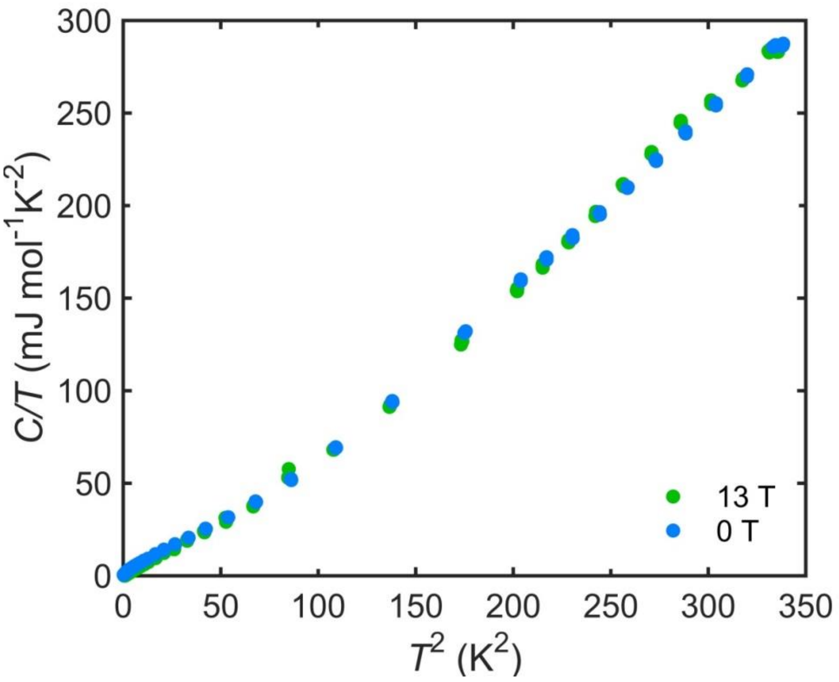


**Figure S13** The specific heat of single crystal $Ba_2CuTeO_6$ at 0 T and 13 T.

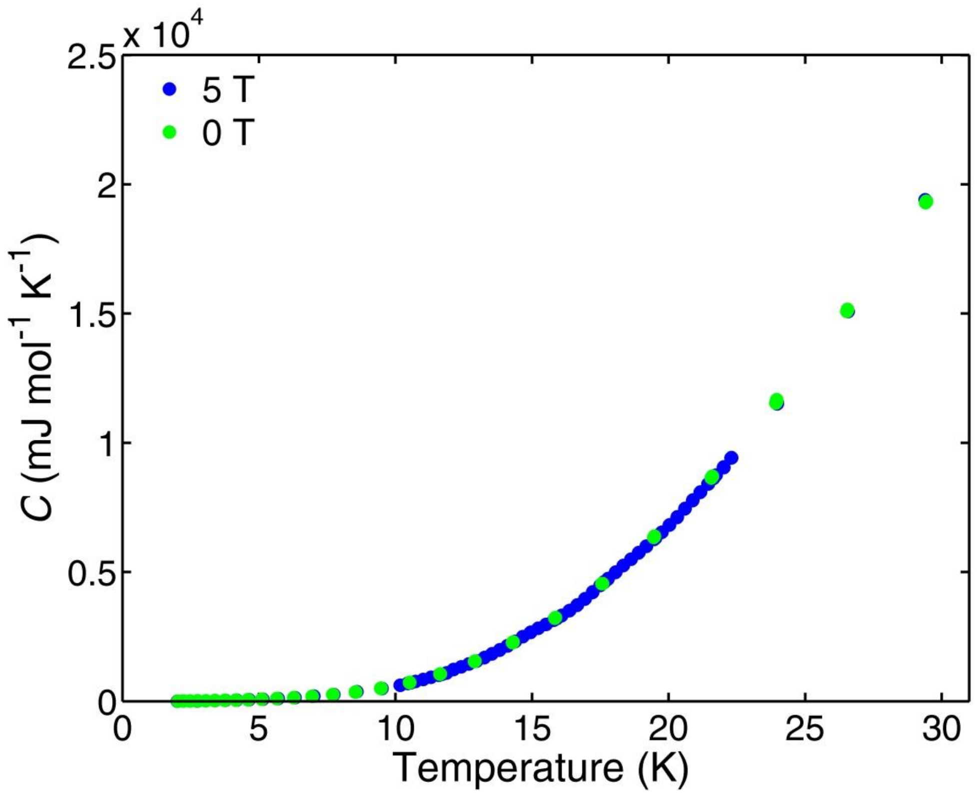


**Figure S14** The specific heat of single crystal $Ba_2CuTeO_6$ at 0 T and 5 T.

**References**:

[1] A. N. Yaresko, A. Y. Perlov, R. Hayn, and H. Rosner, *Phys. Rev. B* **65**, 115111 (2002).
[2] A. N. Yaresko, *Phys. Rev. B* **77**, 115106 (2008).
[3] J. C. Bonner and M. E. Fisher, *Phys. Rev.* **135**, A640 (1964).
[4] W. E. Hatfield, R. R. Weller, and J. W. Hall, *Inorg. Chem*. **19**, 3825 (1980).
[5] D. C. Johnston, M. Troyer, S. Miyahara, D. Lidsky, K. Ueda, M. Azuma, Z. Hiroi, M. Takano, M. Isobe, Y. Ueda, M. A. Korotin, V. I. Anisimov, A. V. Mahajan, and L. L. Miller, (2000), arXiv:cond-mat/0001147 [cond-mat].
